# Supplementary material for: Unscented Orientation Estimation Based on the Bingham Distribution
Source: arXiv:1311.5796 source file (2013-11-22)
Supplement: Supplementary file 1 [file appendix.tex]

\subsection{Introduction} 
%todo: applications

There are different parameterizations for 3D orientations such as rotation matrices, Euler angles, axis/angle representations and unit quaternions \cite{Shuster93}. In this paper, we consider the parameterization through unit quaternions, since they do not suffer from any singularities. The restriction to vectors of unit length is handled by consideration of an estimation problem on the unit hypersphere.

This leaves just one issue: two quaternions $\vec{q}$ and $-\vec{q}$ represent the same rotation. To solve this problem, we consider an antipodally symmetric probability distribution on the unit hypersphere, which assigns the same probability to $\vec{q}$ an $-\vec{q}$. A probability distribution that fulfills these criteria is the Bingham distribution \cite{bingham1974}. It has previously been used in geological applications \cite{kunze2004}.

Traditional approaches to 3D pose estimation are usually based on the assumption of a Gaussian distribution at some point. In some instances, nonlinear filters such as the UKF are applied directly to a state vector that contains some parameterization for rotations (todo cite). More sophisticated approaches include a UKF modified to handle quaternions  \cite{Kraft2003} and the use of projected Gaussian distributions \cite{Feiten09}. These approaches usually run into difficulties when the uncertainty is large because the Gaussian approximation becomes increasingly inaccurate.
%todo cite feiten fusion paper?

\begin{itemize}
\item motivation for quaternions \cite{Shuster93}
\item motivation for Bingham distribution
\item issues with common approaches: linearization, problems with large uncertainties
\end{itemize}

\subsection{Bingham Distribution}

\begin{definition}
Let $S^{d-1} = \{ \vec{x} \in \mathbb{R}^d : ||x|| = 1 \} \subset \mathbb{R}^d$ be the unit hyper sphere in $\mathbb{R}^d$.
A Bingham distribution \cite{bingham1974} with parameters $\mat{M}$ and $\mat{Z}$ has the probability density function
\[ f:S^{d-1}\to \mathbb{R}, \quad f(\vec{x}) = \frac{1}{F} \cdot \exp(\vec{x}^T \mat{M} \mat{Z} \mat{M} T \vec{x}) \ , \]
with normalization constant $F$. We require the orientation matrix $\mat{M} \in \mathbb{R}^{d \times d}$ to be an orthogonal matrix $(\mat{M}\mat{M}^T = \mat{M}^T\mat{M} = \mat{I}_{d \times d})$. Furthermore, we require the concentration matrix $\mat{Z} \in \mathbb{R}^{d \times d}$ to be a diagonal matrix $\mat{Z} = \diag (z_1, \dots z_{d-1}, 0)$ with $z_1 \leq \dots \leq z_{d-1} \leq 0$.
\end{definition}

As is obvious from its definition, the pdf of a Bingham distribution is antipodally symmetric, that is $f(x) = f(-x)$ for all $x \in S^{d-1}$. Thus, a four-dimensional Bingham distribution can be interpreted as a distribution on the unit quaternions, which takes the property into account that $q$ and $-q$ define the same rotation.

The normalization constant F is related to the confluent hypergeometric function of matrix argument \cite{abramowitz1964} according to
\[ F = |S^{d-1}| \cdot {}_1 F_1 \left( \frac{1}{2}, \frac{d}{2}, \mat{Z} \right), \]
where $|S^{d-1}|$ is the surface of the unit sphere in $d$ dimensions. Calculation of the normalization constant is quite difficult \cite{muller2001}. A common solution consists in the use of precomputed lookup-tables \cite{Glover13TR}, \cite{Glover13}. Since this approach requires a large amount of memory, we use the saddle point approximation proposed by Kume et al. \cite{Kume05} instead.
%todo mention \cite{koev2006}

\begin{lemma}
The renormalized product of two Bingham pdfs with parameters $(\mat{M}_1, \mat{Z}_1)$ and $(\mat{M}_2, \mat{Z}_2)$ is obtained from the eigenvalue decomposition of
\[\mat{C} := \mat{M}_1 \mat{Z}_1 \mat{M}_1^T + \mat{M}_2 \mat{Z}_2 \mat{M}_2^T \ .\]
It has parameters $(\mat{M}, \mat{Z})$ where $M$ are the unit eigenvectors of $\mat{C}$, $\mat{D}$ has the eigenvalues of $\mat{C}$ in ascending order on the diagonal and $\mat{Z}=\mat{D}-\mat{D}_{dd} \mat{I}_{d \times d}$, where $D_{dd}$ is the bottom right entry of $\mat{D}$.
\end{lemma}
\begin{proof}
see \cite{Fusion13_Kurz-Bingham} or \cite{Glover13TR}.
\end{proof}

\begin{lemma}
The covariance matrix of a Bingham distribution $(\mat{M}, \mat{Z})$ is given by 
\[ \mat{C} = \mat{M} \cdot \diag \left( \frac{\frac{\partial}{\partial z_1}F}{F}, \dots, \frac{\frac{\partial}{\partial z_d}F}{F} \right) \cdot \mat{M}^T  \]
\end{lemma}
\begin{proof}
see \cite{Fusion13_Kurz-Bingham}.
\end{proof}

\begin{lemma}
\label{lemma:mle}
For a given covariance matrix $\mat{C}$, the parameters $(\mat{M}, \mat{Z})$ of the Bingham distribution with maximum likelihood can be obtained as follows. The orientation $M$ is calculated from the eigendecomposition 
\[  \mat{C}= \mat{M} \cdot \diag (\omega_1, \dots, \omega_d) \cdot \mat{M}^T \ . \]
The concentration $\mat{Z} = \diag  (z_1, \dots, z_d)$ is obtained by solving the system of equations
\[ \frac{  \frac{\partial}{\partial z_i} {}_1F_1 \left( \frac{1}{2}, \frac{d}{2}, \diag (z_1, \dots, z_d) \right)  }{  {}_1F_1 \left( \frac{1}{2}, \frac{d}{2}, \diag (z_1, \dots, z_d)  \right) } = \omega_i, \quad i=1, \dots, d \]
under the constraint $z_d = 0$.
\end{lemma}
\begin{proof}
see \cite{bingham1974}.
\end{proof}

From now on, we restrict our considerations to the quaternion case, i.e., $d=4$. We define a composition function that is analogous to addition of real vectors.

\begin{definition}
The composition function $\oplus: S_3 \times S_3 \to S_3$ is given by quaternion multiplication, i.e.,
\[ 
\begin{pmatrix} x_1 \\ x_2 \\ x_3 \\ x_4 \end{pmatrix}   
\oplus \begin{pmatrix} y_1 \\ y_2 \\ y_3 \\ y_4 \end{pmatrix}   
= 
\begin{pmatrix}
x_1 y_1 - x_2 y_2 - x_3 y_3 - x_4 y_4 \\
x_1 y_2 + x_2 y_1 + x_3 y_4 - x_4 y_3 \\
x_1 y_3 - x_2 y_4 + x_3 y_1 + x_4 y_2 \\
x_1 y_4 + x_2 y_3 - x_3 y_2 + x_4 y_1
\end{pmatrix}
\ . \]
\end{definition}

We now extend the composition operator to Bingham distributed random variables. Bingham distributions are not closed under composition, so we have to rely on an approximation. First, we calculate the covariance matrices of both Bingham distributions. Then we obtain the covariance matrix of the composition as described in \cite{Glover13TR}. Finally, we use Lemma \ref{lemma:mle} to obtain the Bingham distribution with identical covariance.

\subsection{Deterministic Sampling}
%todo avoid using w and omega

For a given covariance matrix $\mat{C}$, we want to obtain samples on the unit hypersphere with the given covariance, i.e., for a matrix $\mat{X}$ of $n$ samples, it holds that
\begin{align*}
\mat{C} = \frac{1}{n} X X^T &= \frac{1}{n} \begin{pmatrix} x_{11} & \cdots & x_{1n} \\ x_{21} & \cdots & x_{2n} \\ x_{31} & \cdots & x_{3n} \\ x_{41} & \cdots & x_{4n}\end{pmatrix} \begin{pmatrix} x_{11} & \cdots & x_{1n} \\ x_{21} & \cdots & x_{2n} \\ x_{31} & \cdots & x_{3n} \\ x_{41} & \cdots & x_{4n}\end{pmatrix}^T
\end{align*}
with $|| (x_{1i}, x_{2i}, x_{3i}, x_{4i} )^T || = 1$ for $i=1, \dots, n$.

Calculating the samples gets easier, if we make some simplifications and restrictions on their form. First of all, we assume that $\mat{M}$ is the identity matrix. If $\mat{M}$ is not the identity, we can subsequently rotate our samples by $\mat{M}$. Thus, the mode is always $\pm (0,\dots, 0, 1)^T$. Then, we parameterize our samples by a small number of parameters, which allows us to easily ensure that the samples are unit vectors.

Consider the seven samples
\[ \mat{X} = \begin{pmatrix}  
0 & \sin(\alpha_1) & -\sin(\alpha_1) & 0           & 0            & 0            & 0 \\ 
0 & 0            & 0             & \sin(\alpha_2) & -\sin(\alpha_2) & 0            & 0 \\
0 & 0            & 0             & 0           & 0            & \sin(\alpha_3) & -\sin(\alpha_3)\\
1 & \cos(\alpha_1) & \cos(\alpha_1)  & \cos(\alpha_2) & \cos(\alpha_2)  & \cos(\alpha_3) & \cos(\alpha_3)\\
\end{pmatrix} \ \]
for angles $\alpha_1, \alpha_2, \alpha_3$. Then, the covariance matrix is
\begin{align*}
\frac{1}{7} \mat{X} \mat{X}^T =& \frac{1}{7} \text{diag} \Big(  2 \sin(\alpha_1)^2, 2\sin(\alpha_2)^2, 2 \sin(\alpha_3)^2, \\
&1 + 2 \cos(\alpha_1)^2+ 2 \cos(\alpha_2)^2+ 2 \cos(\alpha_3)^2  \Big) \ . 
\end{align*}
On the other hand, the covariance matrix of a given Bingham distribution with $\mat{M} = \diag (1,1,1,1)$ is given by $\diag(\omega_1, \omega_2, \omega_3, \omega_4)$. We solve for $\alpha_1, \alpha_2$ and $\alpha_3$, which yields
\begin{align*}
\alpha_i &= \arcsin \left( \sqrt{\frac{7}{2} \omega_i} \right) \ ,  \quad i=1,2,3
\end{align*}
However, this in all cases, because no solution of the above form may not exist. If the uncertainty is very large in one direction and very small in another, then there is no solution where the samples are located on the "axes". This can be solved by weighting the samples differently.

If we consider weighted samples the covariance matrix is 
\[ \mat{X} \mat{W} \mat{X}^T \]
where $W$ is a diagonal matrix with trace $1$. For reasons of symmetry, this leaves three degrees of freedom:
\[ \mat{W} = \text{diag} (1 - 2w_1 - 2w_2 - 2w_3, w_1, w_1, w_2, w_2, w_3, w_3 ) \]
Thus, the covariance matrix is
\begin{align*}
\mat{C} = & \text{diag} \Big( 2 w_1 \sin(\alpha_1)^2, 2 w_2 \sin(\alpha_2)^2, 2 w_3 \sin(\alpha_3)^2, \\
&1-2w_1-2w_2-2w_3 \\ 
&+ 2 w_1 \cos(\alpha_1)^2+ 2 w_2 \cos(\alpha_2)^2+ 2 w_3 \cos(\alpha_3)^2  \Big) \ .
\end{align*}
Solving for $\alpha_1$ yields
\[ 
\alpha_1 = \arcsin \left( \sqrt{\frac{\omega_1}{2 w_1} } \right)
\]
There is a real solution to this equation if
\[ \sqrt{\frac{\omega_1}{2 w_1}} \leq 1 \Rightarrow \left| \frac{\omega_1}{2 w_1} \right| \leq 1 \]
If we restrict ourselves to positive weights and since $\omega_1 >0$ we obtain
\[ \frac{\omega_1}{2 w_1} \leq 1 \Rightarrow \frac{\omega_1}{2} \leq w_1 \]
We choose the weight $w_1 = \max (\frac{1}{7}, \frac{\omega_1}{2} )$. The derivations for $\alpha_2$ and $\alpha_3$ are analogous.

%Is this always well defined or can the sum of weights get larger than $1$? Might it be preferable to choose the weight even larger so the samples move closer together?

\subsection{Nonlinear filter}
filter: predict and update

\begin{algorithm}
\KwIn{estimate, noise}
\KwOut{prediction}
obtain samples\;
propagate samples\;
obtain covariance matrix\;
calculate composition\;
estimate Bingham parameters\;
\caption{Algorithm for prediction.}
\label{algo:prediction}
\end{algorithm}

\begin{algorithm}
\KwIn{prediction, noise}
\KwOut{estimate}
multiply pdfs\;
\caption{Algorithm for update.}
\label{algo:update}
\end{algorithm}

\section{Evaluation}
\begin{itemize}
\item simulations, comparison to QKF
\end{itemize}

\section{Conclusion}
In this paper, we have presented an algorithm for recursive 3D pose estimation. The proposed methods is based on the Bingham distribution and is able to handle a nonlinear system equation by use of deterministic sampling.
